# Supplementary material for: FedAdapter: Efficient Federated Learning for Modern NLP
Source: arXiv:2205.10162 source file (2023-05-08)
Supplement: Supplementary file 1 [file sec-appendix.tex]

\newpage
\section*{Appendix}
\label{sec:appendix}

\mwx{Rationales: move to \ref{sec:design:scheduler}} Figure~\ref{fig:eval-adapter-heatmap} suggests that adapters on the lower layers have a smaller impact than the higher-layers. Removing the adapters from the layers 0 \- 4 on 20news barely affects performance. This indicates that adapters perform well because they automatically prioritize higher layers. Indeed, focusing on the upper layers is a popular strategy in fine- tuning (Howard \& Ruder, 2018). One intuition is that the lower layers extract lower-level features that are shared among tasks, while  the higher layers build features that are unique to different tasks. This relates to our observation that for some tasks, fine-tuning only the top layers outperforms full fine-tuning.

% Please add the following required packages to your document preamble:
% \usepackage{booktabs}
% \usepackage{multirow}
% \usepackage[table,xcdraw]{xcolor}
% If you use beamer only pass "xcolor=table" option, i.e. \documentclass[xcolor=table]{beamer}
\begin{table*}[]
  \footnotesize
    \begin{tabular}{@{}|c|l|ll|ll|ll|ll|@{}}
    \toprule
    \multicolumn{1}{|l|}{\textbf{}} &
      \textbf{} &
      \multicolumn{2}{c|}{\textbf{TC (20news)}} &
      \multicolumn{2}{c|}{\textbf{TC (agnews)}} &
      \multicolumn{2}{c|}{\textbf{TC (semeval)}} &
      \multicolumn{2}{c|}{\textbf{ST (onto)}} \\ \midrule
    \multicolumn{1}{|l|}{\textbf{Bandwidth}} &
      \textbf{Methods} &
      \multicolumn{1}{l|}{acc=0.8} &
      acc=0.7 &
      \multicolumn{1}{l|}{acc=0.9} &
      acc=0.8 &
      \multicolumn{1}{l|}{acc=0.8} &
      acc=0.7 &
      \multicolumn{1}{l|}{f=0.8} &
      f=0.7 \\ \midrule
     &
      Origin &
      \multicolumn{1}{l|}{41.68} &
      7.95 &
      \multicolumn{1}{l|}{13.19} &
      1.55 &
      \multicolumn{1}{l|}{76.98} &
      16.34 &
      \multicolumn{1}{l|}{305.71} &
      48.18 \\ \cmidrule(l){2-10} 
     &
      Freeze &
      \multicolumn{1}{l|}{16.92} &
      2.38 &
      \multicolumn{1}{l|}{4.66} &
      0.07 &
      \multicolumn{1}{l|}{32.36} &
      7.77 &
      \multicolumn{1}{l|}{199.23} &
      27.29 \\ \cmidrule(l){2-10} 
    \multirow{-3}{*}{1} &
      Adaptive &
      \multicolumn{1}{l|}{{\color[HTML]{FE0000} 2.72}} &
      {\color[HTML]{FE0000} 0.25} &
      \multicolumn{1}{l|}{{\color[HTML]{FE0000} 0.94}} &
      {\color[HTML]{FE0000} 0.01} &
      \multicolumn{1}{l|}{{\color[HTML]{FE0000} 3.54}} &
      {\color[HTML]{FE0000} 1.01} &
      \multicolumn{1}{l|}{{\color[HTML]{FE0000} 45.77}} &
      {\color[HTML]{FE0000} 6.63} \\ \midrule
     &
      Origin &
      \multicolumn{1}{l|}{21.73} &
      4.10 &
      \multicolumn{1}{l|}{6.83} &
      0.84 &
      \multicolumn{1}{l|}{40.30} &
      8.63 &
      \multicolumn{1}{l|}{159.63} &
      25.31 \\ \cmidrule(l){2-10} 
     &
      Freeze &
      \multicolumn{1}{l|}{9.52} &
      1.36 &
      \multicolumn{1}{l|}{2.62} &
      0.05 &
      \multicolumn{1}{l|}{17.56} &
      4.18 &
      \multicolumn{1}{l|}{107.76} &
      14.83 \\ \cmidrule(l){2-10} 
    \multirow{-3}{*}{2} &
      Adaptive &
      \multicolumn{1}{l|}{{\color[HTML]{FE0000} 2.58}} &
      {\color[HTML]{FE0000} 0.22} &
      \multicolumn{1}{l|}{{\color[HTML]{FE0000} 0.88}} &
      {\color[HTML]{FE0000} 0.01} &
      \multicolumn{1}{l|}{{\color[HTML]{FE0000} 3.13}} &
      {\color[HTML]{FE0000} 0.99} &
      \multicolumn{1}{l|}{{\color[HTML]{FE0000} 43.03}} &
      {\color[HTML]{FE0000} 6.42} \\ \midrule
     &
      Origin &
      \multicolumn{1}{l|}{11.91} &
      2.22 &
      \multicolumn{1}{l|}{3.64} &
      0.44 &
      \multicolumn{1}{l|}{21.78} &
      4.65 &
      \multicolumn{1}{l|}{85.55} &
      13.53 \\ \cmidrule(l){2-10} 
     &
      Freeze &
      \multicolumn{1}{l|}{5.97} &
      0.82 &
      \multicolumn{1}{l|}{1.61} &
      0.03 &
      \multicolumn{1}{l|}{10.04} &
      2.50 &
      \multicolumn{1}{l|}{61.24} &
      8.41 \\ \cmidrule(l){2-10} 
    \multirow{-3}{*}{4} &
      Adaptive &
      \multicolumn{1}{l|}{{\color[HTML]{FE0000} 2.34}} &
      {\color[HTML]{FE0000} 0.22} &
      \multicolumn{1}{l|}{{\color[HTML]{FE0000} 0.82}} &
      {\color[HTML]{FE0000} 0.01} &
      \multicolumn{1}{l|}{{\color[HTML]{FE0000} 3.06}} &
      {\color[HTML]{FE0000} 0.94} &
      \multicolumn{1}{l|}{{\color[HTML]{FE0000} 40.92}} &
      {\color[HTML]{FE0000} 6.12} \\ \midrule
     &
      Origin &
      \multicolumn{1}{l|}{6.86} &
      1.19 &
      \multicolumn{1}{l|}{2.09} &
      0.27 &
      \multicolumn{1}{l|}{12.54} &
      2.61 &
      \multicolumn{1}{l|}{48.88} &
      7.70 \\ \cmidrule(l){2-10} 
     &
      Freeze &
      \multicolumn{1}{l|}{4.18} &
      0.55 &
      \multicolumn{1}{l|}{1.16} &
      0.02 &
      \multicolumn{1}{l|}{6.29} &
      1.57 &
      \multicolumn{1}{l|}{{\color[HTML]{FE0000} 38.50}} &
      {\color[HTML]{FE0000} 5.28} \\ \cmidrule(l){2-10} 
    \multirow{-3}{*}{8} &
      Adaptive &
      \multicolumn{1}{l|}{{\color[HTML]{FE0000} 2.14}} &
      {\color[HTML]{FE0000} 0.19} &
      \multicolumn{1}{l|}{{\color[HTML]{FE0000} 0.77}} &
      {\color[HTML]{FE0000} 0.01} &
      \multicolumn{1}{l|}{{\color[HTML]{FE0000} 3.04}} &
      {\color[HTML]{FE0000} 0.84} &
      \multicolumn{1}{l|}{39.33} &
      5.77 \\ \bottomrule
    \end{tabular}
    \caption{BandWidth Heterogeneity. Device: Hybrid}
    \label{tab: eval-bandwidth-heterogenity}
    \end{table*}

% Please add the following required packages to your document preamble:
% \usepackage{booktabs}
% \usepackage{multirow}
% \usepackage[table,xcdraw]{xcolor}
% If you use beamer only pass "xcolor=table" option, i.e. \documentclass[xcolor=table]{beamer}
\begin{table*}[]
  \footnotesize
    \begin{tabular}{@{}|c|l|ll|ll|ll|ll|@{}}
    \toprule
    \multicolumn{1}{|l|}{\textbf{}} &
      \textbf{} &
      \multicolumn{2}{c|}{\textbf{TC (20news)}} &
      \multicolumn{2}{c|}{\textbf{TC (agnews)}} &
      \multicolumn{2}{c|}{\textbf{TC (semeval)}} &
      \multicolumn{2}{c|}{\textbf{ST (onto)}} \\ \midrule
    \multicolumn{1}{|l|}{\textbf{Device}} &
      \textbf{Methods} &
      \multicolumn{1}{l|}{acc=0.8} &
      acc=0.7 &
      \multicolumn{1}{l|}{acc=0.9} &
      acc=0.8 &
      \multicolumn{1}{l|}{acc=0.8} &
      acc=0.7 &
      \multicolumn{1}{l|}{f=0.8} &
      f=0.7 \\ \midrule
     &
      Origin &
      \multicolumn{1}{l|}{40.75} &
      7.70 &
      \multicolumn{1}{l|}{12.83} &
      1.51 &
      \multicolumn{1}{l|}{75.16} &
      16.00 &
      \multicolumn{1}{l|}{298.22} &
      47.09 \\ \cmidrule(l){2-10} 
     &
      Freeze &
      \multicolumn{1}{l|}{15.52} &
      2.12 &
      \multicolumn{1}{l|}{4.19} &
      0.07 &
      \multicolumn{1}{l|}{30.79} &
      7.40 &
      \multicolumn{1}{l|}{189.73} &
      25.99 \\ \cmidrule(l){2-10} 
    \multirow{-3}{*}{TX2} &
      Adaptive &
      \multicolumn{1}{l|}{{\color[HTML]{FE0000} 1.28}} &
      {\color[HTML]{FE0000} 0.12} &
      \multicolumn{1}{l|}{{\color[HTML]{FE0000} 0.44}} &
      {\color[HTML]{FE0000} 0.01} &
      \multicolumn{1}{l|}{{\color[HTML]{FE0000} 1.68}} &
      {\color[HTML]{FE0000} 0.47} &
      \multicolumn{1}{l|}{{\color[HTML]{FE0000} 22.01}} &
      {\color[HTML]{FE0000} 3.19} \\ \midrule
     &
      Origin &
      \multicolumn{1}{l|}{51.16} &
      9.66 &
      \multicolumn{1}{l|}{16.11} &
      1.89 &
      \multicolumn{1}{l|}{94.37} &
      20.09 &
      \multicolumn{1}{l|}{374.43} &
      59.12 \\ \cmidrule(l){2-10} 
     &
      Freeze &
      \multicolumn{1}{l|}{30.11} &
      4.12 &
      \multicolumn{1}{l|}{8.14} &
      0.14 &
      \multicolumn{1}{l|}{46.17} &
      11.09 &
      \multicolumn{1}{l|}{284.53} &
      38.98 \\ \cmidrule(l){2-10} 
    \multirow{-3}{*}{RPI} &
      Adaptive &
      \multicolumn{1}{l|}{{\color[HTML]{FE0000} 15.16}} &
      {\color[HTML]{FE0000} 1.40} &
      \multicolumn{1}{l|}{{\color[HTML]{FE0000} 5.25}} &
      {\color[HTML]{FE0000} 0.07} &
      \multicolumn{1}{l|}{{\color[HTML]{FE0000} 19.45}} &
      {\color[HTML]{FE0000} 5.46} &
      \multicolumn{1}{l|}{{\color[HTML]{FE0000} 258.52}} &
      {\color[HTML]{FE0000} 37.89} \\ \midrule
     &
      Origin &
      \multicolumn{1}{l|}{43.38} &
      8.25 &
      \multicolumn{1}{l|}{13.83} &
      1.65 &
      \multicolumn{1}{l|}{80.17} &
      16.96 &
      \multicolumn{1}{l|}{316.15} &
      49.99 \\ \cmidrule(l){2-10} 
     &
      Freeze &
      \multicolumn{1}{l|}{19.31} &
      2.63 &
      \multicolumn{1}{l|}{5.33} &
      0.09 &
      \multicolumn{1}{l|}{34.90} &
      8.23 &
      \multicolumn{1}{l|}{212.91} &
      29.07 \\ \cmidrule(l){2-10} 
    \multirow{-3}{*}{Straggler} &
      Adaptive &
      \multicolumn{1}{l|}{{\color[HTML]{FE0000} 4.96}} &
      {\color[HTML]{FE0000} 0.47} &
      \multicolumn{1}{l|}{{\color[HTML]{FE0000} 1.84}} &
      {\color[HTML]{FE0000} 0.02} &
      \multicolumn{1}{l|}{{\color[HTML]{FE0000} 6.45}} &
      {\color[HTML]{FE0000} 1.68} &
      \multicolumn{1}{l|}{{\color[HTML]{FE0000} 79.63}} &
      {\color[HTML]{FE0000} 11.55} \\ \bottomrule
    \end{tabular}
    \caption{Device Heterogeneity. BW: 1MB/s}
    \label{tab: eval-device-heterogenity}
    \end{table*}

\begin{figure}[t]
    \includegraphics[width=0.38\textwidth]{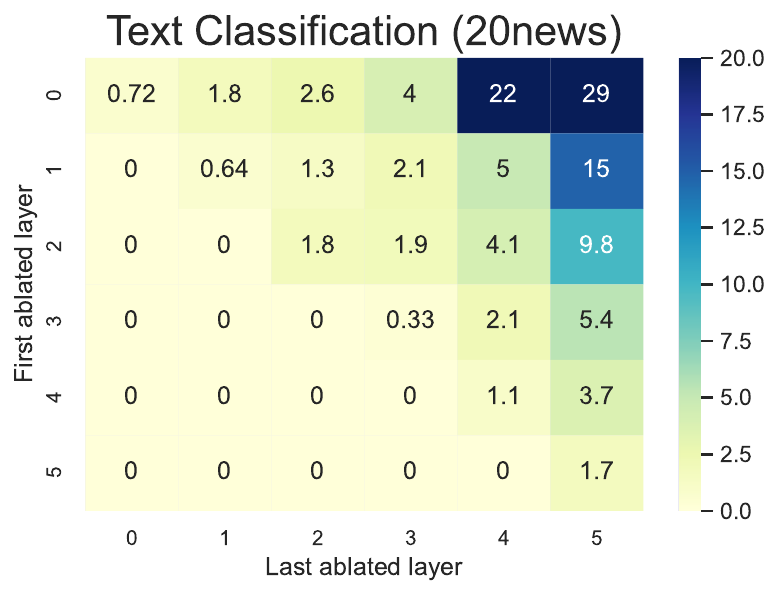}
    \caption{Ablation of trained adapters from continuous layer spans. }
    \label{fig:eval-adapter-heatmap}
\end{figure}

% The heatmap shows the relative decrease in validation accuracy to the fully trained adapted model. The y and x axes indicate the first and last layers ablated (inclusive), respectively. The diagonal cells, indicate ablation of a single layer's adapters. The cell in the top-right indicates ablation of all adapters. Cells in the lower triangle are meaningless, and are set to 0\%, the best possible relative performance.

% \begin{figure}[t]
%     \centering
%     \begin{minipage}[b]{0.24\textwidth}
%         \includegraphics[width=1.0\textwidth]{figs/eval-heatmap-TC.pdf}
%         \subcaption{Uniform}
%     \end{minipage}
%     ~
%     \begin{minipage}[b]{0.24\textwidth}
%         \includegraphics[width=1.0\textwidth]{figs/eval-heatmap-ST.pdf}
%         \subcaption{Non-iid}
%     \end{minipage}
%     \caption{Ablation of trained adapters from continuous layer spans. The heatmap shows the relative decrease in validation accuracy to the fully trained adapted model. The y and x axes indicate the first and last layers ablated (inclusive), respectively. The diagonal cells, indicate ablation of a single layer's adapters. The cell in the top-right indicates ablation of all adapters. Cells in the lower triangle are meaningless, and are set to 0\%, the best possible relative performance.}
%     \label{fig:eval-adapter-heatmap}
% \end{figure}
